# Supplementary material for: Axion-mediated electron-nucleus and electron-electron interactions in barium monofluoride molecule
Source: arXiv:2404.05065 source file (2024-04-07)
Supplement: Supplementary file 1 [file Supplementary.pdf]

# Supplementary: Axion-mediated electron-nucleus and electron-electron interactions in barium monofluoride molecule


Sergey D. Prosnyak[1, 2, *] and Leonid V. Skripnikov[1, 2, †]

[1] Petersburg Nuclear Physics Institute named by B.P. Konstantinov of National Research Centre "Kurchatov Institute", Gatchina, Leningrad District 188300, Russia

[2] Saint Petersburg State University, 7/9 Universitetskaya nab., St. Petersburg, 199034 Russia



(Dated: 02.04.2024)


TABLE I. Values of molecular parameters $W_{\text{ax}}^{(eN)}(m_a)$ for the $\text{HfF}^+$ molecular cation using the Eq. (2) of the main text at various levels of electronic structure theory (published in our previous paper [1]). The "Final" column is the sum of CCSD(T) results and corrections described in the main text of Ref. [1]. The last column provides limits on $|\bar{g}_N^s g_e^p|$ derived from the experimental data [2] corresponding to the ALP masses given in the first column.

| $m_a$, eV | $W_{\text{ax}}^{(eN)}(m_a)$, $m_e c/\hbar$ | | | | $\lvert\bar{g}_N^s g_e^p\rvert$ limit, $\hbar c$ |
|---|---|---|---|---|---|
| | DHF | CCSD | CCSD(T) | Final | |
| 1 | $+1.20 \cdot 10^{-5}$ | $+1.72 \cdot 10^{-5}$ | $+1.68 \cdot 10^{-5}$ | $+1.67 \cdot 10^{-5}$ | $1.11 \cdot 10^{-20}$ |
| 10 | $+1.20 \cdot 10^{-5}$ | $+1.72 \cdot 10^{-5}$ | $+1.68 \cdot 10^{-5}$ | $+1.67 \cdot 10^{-5}$ | $1.11 \cdot 10^{-20}$ |
| $10^2$ | $+1.19 \cdot 10^{-5}$ | $+1.73 \cdot 10^{-5}$ | $+1.68 \cdot 10^{-5}$ | $+1.66 \cdot 10^{-5}$ | $1.11 \cdot 10^{-20}$ |
| $10^3$ | $+1.14 \cdot 10^{-5}$ | $+1.60 \cdot 10^{-5}$ | $+1.56 \cdot 10^{-5}$ | $+1.54 \cdot 10^{-5}$ | $1.19 \cdot 10^{-20}$ |
| $10^4$ | $+2.87 \cdot 10^{-6}$ | $+3.59 \cdot 10^{-6}$ | $+3.55 \cdot 10^{-6}$ | $+3.30 \cdot 10^{-6}$ | $5.25 \cdot 10^{-20}$ |
| $10^5$ | $-8.36 \cdot 10^{-6}$ | $-1.14 \cdot 10^{-5}$ | $-1.12 \cdot 10^{-5}$ | $-1.15 \cdot 10^{-5}$ | $1.66 \cdot 10^{-20}$ |
| $10^6$ | $-3.88 \cdot 10^{-6}$ | $-6.43 \cdot 10^{-6}$ | $-6.27 \cdot 10^{-6}$ | $-6.41 \cdot 10^{-6}$ | $2.97 \cdot 10^{-20}$ |
| $10^7$ | $-1.72 \cdot 10^{-7}$ | $-2.86 \cdot 10^{-7}$ | $-2.79 \cdot 10^{-7}$ | $-2.85 \cdot 10^{-7}$ | $6.67 \cdot 10^{-19}$ |
| $10^8$ | $-3.19 \cdot 10^{-9}$ | $-5.33 \cdot 10^{-9}$ | $-5.19 \cdot 10^{-9}$ | $-5.30 \cdot 10^{-9}$ | $3.59 \cdot 10^{-17}$ |
| $10^9$ | $-3.53 \cdot 10^{-11}$ | $-5.90 \cdot 10^{-11}$ | $-5.74 \cdot 10^{-11}$ | $-5.85 \cdot 10^{-11}$ | $3.24 \cdot 10^{-15}$ |
| $10^{10}$ | $-3.54 \cdot 10^{-13}$ | $-5.91 \cdot 10^{-13}$ | $-5.75 \cdot 10^{-13}$ | $-5.87 \cdot 10^{-13}$ | $3.24 \cdot 10^{-13}$ |

TABLE II. Values of molecular parameters $W_{\text{ax}}^{(eN)}(m_a)$ for the $\text{HfF}^+$ molecular cation using the Eq. (1) of the main text at various levels of electronic structure theory. In these calculations we used the same approach, as in Ref. [1]. The last column provides limits on $|\bar{g}_N^s g_e^p|$ derived from the experimental data [2] corresponding to the ALP masses given in the first column.

| $m_a$, eV | $W_{\text{ax}}^{(eN)}(m_a)$, $m_e c/\hbar$ | | | | $\lvert\bar{g}_N^s g_e^p\rvert$ limit, $\hbar c$ |
|---|---|---|---|---|---|
| | DHF | CCSD | CCSD(T) | Final | |
| 1 | $+1.20 \cdot 10^{-5}$ | $+1.72 \cdot 10^{-5}$ | $+1.68 \cdot 10^{-5}$ | $+1.67 \cdot 10^{-5}$ | $1.11 \cdot 10^{-20}$ |
| 10 | $+1.20 \cdot 10^{-5}$ | $+1.72 \cdot 10^{-5}$ | $+1.68 \cdot 10^{-5}$ | $+1.67 \cdot 10^{-5}$ | $1.11 \cdot 10^{-20}$ |
| $10^2$ | $+1.19 \cdot 10^{-5}$ | $+1.73 \cdot 10^{-5}$ | $+1.68 \cdot 10^{-5}$ | $+1.66 \cdot 10^{-5}$ | $1.11 \cdot 10^{-20}$ |
| $10^3$ | $+1.14 \cdot 10^{-5}$ | $+1.60 \cdot 10^{-5}$ | $+1.56 \cdot 10^{-5}$ | $+1.54 \cdot 10^{-5}$ | $1.19 \cdot 10^{-20}$ |
| $10^4$ | $+2.87 \cdot 10^{-6}$ | $+3.59 \cdot 10^{-6}$ | $+3.55 \cdot 10^{-6}$ | $+3.30 \cdot 10^{-6}$ | $5.25 \cdot 10^{-20}$ |
| $10^5$ | $-8.36 \cdot 10^{-6}$ | $-1.14 \cdot 10^{-5}$ | $-1.12 \cdot 10^{-5}$ | $-1.15 \cdot 10^{-5}$ | $1.66 \cdot 10^{-20}$ |
| $10^6$ | $-3.87 \cdot 10^{-6}$ | $-6.43 \cdot 10^{-6}$ | $-6.26 \cdot 10^{-6}$ | $-6.41 \cdot 10^{-6}$ | $2.97 \cdot 10^{-20}$ |
| $10^7$ | $-1.70 \cdot 10^{-7}$ | $-2.83 \cdot 10^{-7}$ | $-2.76 \cdot 10^{-7}$ | $-2.82 \cdot 10^{-7}$ | $6.74 \cdot 10^{-19}$ |
| $10^8$ | $-2.90 \cdot 10^{-9}$ | $-4.84 \cdot 10^{-9}$ | $-4.71 \cdot 10^{-9}$ | $-4.81 \cdot 10^{-9}$ | $3.95 \cdot 10^{-17}$ |
| $10^9$ | $-3.07 \cdot 10^{-11}$ | $-5.12 \cdot 10^{-11}$ | $-4.99 \cdot 10^{-11}$ | $-5.09 \cdot 10^{-11}$ | $3.73 \cdot 10^{-15}$ |
| $10^{10}$ | $-3.07 \cdot 10^{-13}$ | $-5.13 \cdot 10^{-13}$ | $-5.00 \cdot 10^{-13}$ | $-5.10 \cdot 10^{-13}$ | $3.73 \cdot 10^{-13}$ |


* prosnyak_sd@pnpi.nrcki.ru, prosnyak.sergey@yandex.ru

TABLE III. Values of molecular parameters $W_{\mathrm{ax}}^{(eN)}(m_a)$ for BaF (in units of $m_e c/\hbar$) obtained at different levels of electronic structure theory using the AE2Z basis set.

| $m_a$, eV | DHF | CCSD | CCSD(T) |
|---|---|---|---|
| 1 | $+1.41 \cdot 10^{-5}$ | $+1.82 \cdot 10^{-5}$ | $+1.79 \cdot 10^{-5}$ |
| 10 | $+1.41 \cdot 10^{-5}$ | $+1.82 \cdot 10^{-5}$ | $+1.79 \cdot 10^{-5}$ |
| $10^2$ | $+1.40 \cdot 10^{-5}$ | $+1.81 \cdot 10^{-5}$ | $+1.78 \cdot 10^{-5}$ |
| $10^3$ | $+1.11 \cdot 10^{-5}$ | $+1.51 \cdot 10^{-5}$ | $+1.49 \cdot 10^{-5}$ |
| $10^4$ | $+1.28 \cdot 10^{-6}$ | $+1.86 \cdot 10^{-6}$ | $+1.83 \cdot 10^{-6}$ |
| $10^5$ | $-6.94 \cdot 10^{-6}$ | $-1.13 \cdot 10^{-5}$ | $-1.11 \cdot 10^{-5}$ |
| $10^6$ | $-3.19 \cdot 10^{-6}$ | $-4.97 \cdot 10^{-6}$ | $-4.88 \cdot 10^{-6}$ |
| $10^7$ | $-9.12 \cdot 10^{-8}$ | $-1.42 \cdot 10^{-7}$ | $-1.40 \cdot 10^{-7}$ |
| $10^8$ | $-1.19 \cdot 10^{-9}$ | $-1.85 \cdot 10^{-9}$ | $-1.82 \cdot 10^{-9}$ |
| $10^9$ | $-1.21 \cdot 10^{-11}$ | $-1.89 \cdot 10^{-11}$ | $-1.85 \cdot 10^{-11}$ |
| $10^{10}$ | $-1.21 \cdot 10^{-13}$ | $-1.89 \cdot 10^{-13}$ | $-1.86 \cdot 10^{-13}$ |

TABLE IV. Values of molecular parameters $W_{\mathrm{ax}}^{(eN)}(m_a)$ for BaF (in units of $m_e c/\hbar$) using the Eq. (2) of the main text obtained at different levels of electronic structure theory.

| $m_a$, eV | DHF | CCSD | CCSD(T) |
|---|---|---|---|
| 1 | $+1.41 \cdot 10^{-5}$ | $+1.77 \cdot 10^{-5}$ | $+1.74 \cdot 10^{-5}$ |
| 10 | $+1.41 \cdot 10^{-5}$ | $+1.77 \cdot 10^{-5}$ | $+1.74 \cdot 10^{-5}$ |
| $10^2$ | $+1.40 \cdot 10^{-5}$ | $+1.77 \cdot 10^{-5}$ | $+1.73 \cdot 10^{-5}$ |
| $10^3$ | $+1.11 \cdot 10^{-5}$ | $+1.48 \cdot 10^{-5}$ | $+1.45 \cdot 10^{-5}$ |
| $10^4$ | $+1.27 \cdot 10^{-6}$ | $+1.89 \cdot 10^{-6}$ | $+1.86 \cdot 10^{-6}$ |
| $10^5$ | $-6.93 \cdot 10^{-6}$ | $-1.09 \cdot 10^{-5}$ | $-1.07 \cdot 10^{-5}$ |
| $10^6$ | $-3.19 \cdot 10^{-6}$ | $-4.79 \cdot 10^{-6}$ | $-4.70 \cdot 10^{-6}$ |
| $10^7$ | $-9.25 \cdot 10^{-8}$ | $-1.39 \cdot 10^{-7}$ | $-1.36 \cdot 10^{-7}$ |
| $10^8$ | $-1.35 \cdot 10^{-9}$ | $-2.02 \cdot 10^{-9}$ | $-1.99 \cdot 10^{-9}$ |
| $10^9$ | $-1.42 \cdot 10^{-11}$ | $-2.12 \cdot 10^{-11}$ | $-2.09 \cdot 10^{-11}$ |
| $10^{10}$ | $-1.42 \cdot 10^{-13}$ | $-2.13 \cdot 10^{-13}$ | $-2.09 \cdot 10^{-13}$ |

† skripnikov_lv@pnpi.nrcki.ru,
leonidos239@gmail.com; http://www.qchem.pnpi.spb.ru

[1] S. D. Prosnyak, D. E. Maison, and L. V. Skripnikov, Symmetry **15** (2023), 10.3390/sym15051043.
[2] T. S. Roussy, L. Caldwell, T. Wright, W. B. Cairncross, Y. Shagam, K. B. Ng, N. Schlossberger, S. Y. Park, A. Wang, J. Ye, and E. A. Cornell, Science **381**, 46 (2023).
